# Supplementary material for: Water on hexagonal boron nitride from diffusion Monte Carlo
Source: arXiv:1505.03291 source file (2015-05-13)
Supplement: Supplementary file 1 [file supporting_info.pdf]

# Water on hexagonal boron nitride from diffusion Monte Carlo

Yasmine S. Al-Hamdani,[1,2] Ming Ma,[1,2] Dario Alfè,[1,3] O. Anatole von Lilienfeld,[4,5] and Angelos Michaelides[1,2,a)]

[1)] *Thomas Young Centre and London Centre for Nanotechnology, 17–19 Gordon Street, London, WC1H 0AH, U.K.*

[2)] *Department of Chemistry, University College London, 20 Gordon Street, London, WC1H 0AJ, U.K.*

[3)] *Department of Earth Sciences, University College London, Gower Street, London WC1E 6BT, U.K.*

[4)] *Institute of Physical Chemistry and National Center for Computational Design and Discovery of Novel Materials, Department of Chemistry, University of Basel, Klingelbergstrasse 80 CH-4056 Basel, Switzerland*

[5)] *Argonne Leadership Computing Facility, Argonne National Laboratories, 9700 S. Cass Avenue Argonne, Illinois 60439, USA*

(Dated: 31 March 2015)

Here we have included the structural coordinates for two different adsorption sites of a water monomer on h-BN.

[a)]Electronic mail: angelos.michaelides@ucl.ac.uk

TABLE S1. Water adsorbed above an N site of h-BN with an oxygen-surface distance of 3.20 Å. Coordinates in xyz format.

| Atom | x | y | z |
|---|---|---|---|
| H | 5.88 | 3.46 | 5.72 |
| H | 6.39 | 3.63 | 4.27 |
| O | 6.66 | 3.73 | 5.20 |
| B | 1.29 | 0.70 | 2.00 |
| B | 2.55 | 2.87 | 2.00 |
| B | 3.81 | 5.05 | 2.00 |
| B | 5.06 | 7.22 | 2.00 |
| B | 3.81 | 0.70 | 2.00 |
| B | 5.06 | 2.87 | 2.00 |
| B | 6.32 | 5.05 | 2.00 |
| B | 7.57 | 7.22 | 2.00 |
| B | 6.32 | 0.70 | 2.00 |
| B | 7.57 | 2.87 | 2.00 |
| B | 8.83 | 5.05 | 2.00 |
| B | 10.09 | 7.22 | 2.00 |
| B | 8.83 | 0.70 | 2.00 |
| B | 10.09 | 2.87 | 2.00 |
| B | 11.34 | 5.05 | 2.00 |
| B | 12.60 | 7.22 | 2.00 |
| N | 2.55 | 1.42 | 2.00 |
| N | 3.81 | 3.60 | 2.00 |
| N | 5.06 | 5.77 | 2.00 |
| N | 6.32 | 7.95 | 2.00 |
| N | 5.06 | 1.42 | 2.00 |
| N | 6.32 | 3.60 | 2.00 |
| N | 7.57 | 5.77 | 2.00 |
| N | 8.83 | 7.95 | 2.00 |
| N | 7.57 | 1.42 | 2.00 |
| N | 8.83 | 3.60 | 2.00 |
| N | 10.09 | 5.77 | 2.00 |
| N | 11.34 | 7.95 | 2.00 |
| N | 10.09 | 1.42 | 2.00 |
| N | 11.34 | 3.60 | 2.00 |
| N | 12.60 | 5.77 | 2.00 |
| N | 13.85 | 7.95 | 2.00 |

TABLE S2. Water adsorbed above a B site of h-BN with an oxygen-surface distance of 3.20 Å. Coordinates in xyz format.

| Atom | x | y | z |
|---|---|---|---|
| H | 8.42 | 2.79 | 5.45 |
| H | 6.89 | 2.80 | 5.68 |
| O | 7.60 | 3.26 | 5.20 |
| B | 1.29 | 0.70 | 2.00 |
| B | 2.55 | 2.87 | 2.00 |
| B | 3.81 | 5.05 | 2.00 |
| B | 5.06 | 7.22 | 2.00 |
| B | 3.81 | 0.70 | 2.00 |
| B | 5.06 | 2.87 | 2.00 |
| B | 6.32 | 5.05 | 2.00 |
| B | 7.57 | 7.22 | 2.00 |
| B | 6.32 | 0.70 | 2.00 |
| B | 7.57 | 2.87 | 2.00 |
| B | 8.83 | 5.05 | 2.00 |
| B | 10.09 | 7.22 | 2.00 |
| B | 8.83 | 0.70 | 2.00 |
| B | 10.09 | 2.87 | 2.00 |
| B | 11.34 | 5.05 | 2.00 |
| B | 12.60 | 7.22 | 2.00 |
| N | 2.55 | 1.42 | 2.00 |
| N | 3.81 | 3.60 | 2.00 |
| N | 5.06 | 5.77 | 2.00 |
| N | 6.32 | 7.95 | 2.00 |
| N | 5.06 | 1.42 | 2.00 |
| N | 6.32 | 3.60 | 2.00 |
| N | 7.57 | 5.77 | 2.00 |
| N | 8.83 | 7.95 | 2.00 |
| N | 7.57 | 1.42 | 2.00 |
| N | 8.83 | 3.60 | 2.00 |
| N | 10.09 | 5.77 | 2.00 |
| N | 11.34 | 7.95 | 2.00 |
| N | 10.09 | 1.42 | 2.00 |
| N | 11.34 | 3.60 | 2.00 |
| N | 12.60 | 5.77 | 2.00 |
| N | 13.85 | 7.95 | 2.00 |
